# Supplementary material for: How wet should be the reaction coordinate for ligand unbinding?
Source: arXiv:1605.07090 ancillary file (2016-05-23)
Supplement: Supplementary file 1 [file si.pdf]

# Supplemental Information: How wet should be the reaction coordinate for ligand unbinding?

Pratyush Tiwary[1] and B. J. Berne[1,*]
[1]Department of Chemistry, Columbia University, New York 10027, USA.
(Dated: May 23, 2016)

## I. SYSTEM DETAILS

The model ligand used in this work is a $C_{60}$ fullerene and the pocket is an ellipsoidal cavity carved from a hydrophobic slab, all interacting via Lennard-Jones potentials and enclosed by a periodic box with explicit water and cubic edge length 5.96 nm. This system was introduced previously in works such as Ref. 1, 2. The pocket sites are fixed and interact with the model ligand with a Lennard-Jones site-site potential having $\sigma = 0.4152$ nm, kept the same for all interactions. The pocket itself comprises 2 types of atomic species, interacting with the ligand atoms (color red in Fig. 1 in main text) as described below. The system comprised a total of 34296 atoms, with the total number of ligand, cavity and solvent atoms equaling 60, 9020 and 25216 respectively.

1. cavity atoms (color orange in Fig. 1 in main text), with Lennard-Jones $\epsilon$=0.008 kJ/mol.

2. wall atoms (color blue in Fig. 1 in main text), with Lennard-Jones $\epsilon$=0.0024 kJ/mol.

The solute-solvent interactions are represented by the geometric mean of the respective water and solute parameters, in accordance with the OPLS formalism[3]. All simulations are performed in explicit TIP4P water [4] with the GROMACS 4.5.4 MD package[5], patched with the PLUMED plugin[6]. During the equilibration stage, temperature and pressure are controlled with the stochastic velocity rescaling thermostat [7] and Berendsen barostat[8]. The production runs were NVT (constant number, volume, temperature) with a temperature of 300 K. The PLUMED plugin [6] was used to carry out metadynamics calculations. An integration time-step of $2fs$ was used for all runs.

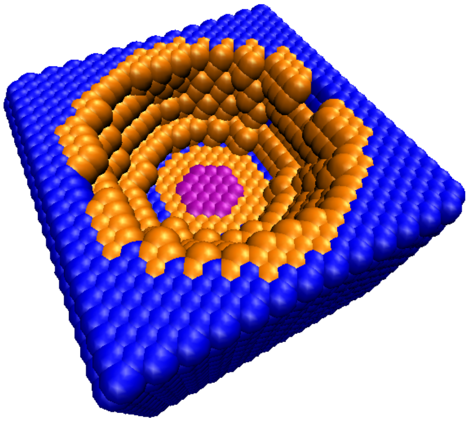

**FIG. 1:** Orange: cavity atoms that interact with the ligand and with water molecules. Blue: wall atoms. The purple colored patch shows the atoms used to calculate the solvation state of the pocket in Eq. 1.

*Electronic address: bb8@columbia.edu

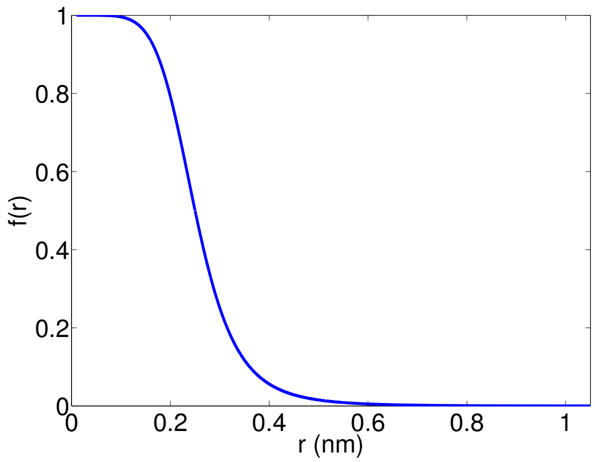


**FIG. 2:** Switching function used in Eq. 1.

## II. DEFINITION OF ORDER PARAMETERS

The following collective variables (CVs) were considered in this work:

1. $z$, which denotes the $z-$coordinate of the centres of masses of (a) the ligand, and (b) the cavity and wall atoms (Fig. 1 in main text). This CV was the same for both the cases, viz. ligand sterically constrained or ligand free to move.

2. $\rho \equiv \sqrt{x^2 + y^2}$, which denotes the separation of the ligand's centre of mass from the z-axis. This CV was applicable only for the case when the ligand was free to move.

3. $w$, which represents the number of water molecules in the cavity. Since we need to this to be smoothly differentiable, we used the following definition for $w$ as implemented in the software PLUMED [6]:

$$w = \sum_{i \in A} \sum_{j \in B} f(r_{i,j}) \tag{1}$$

Here the set $A$ denotes the central patch of the cavity atoms, marked in color purple in Fig. 1. Te set $B$ comprises all the oxygen atoms of the various water molecules. $r_{i,j}$ is the distance in $nm$ between atoms $i$ and $j$ coming from these two sets respectively. The function

$$f(r) \equiv \frac{\left(1 - (r/0.25)^6\right)}{\left(1 - (r/0.25)^{12}\right)} \tag{2}$$

is a switching function that makes $w$ smoothly differentiable. Fig. 2 gives a plot of this function.

## III. SIMULATION DETAILS FOR METADYNAMICS

In this section we provide details of collective variables, biaising kernel, biasing frequency and well-tempered metadynamics bias factor for various cases. This is divided into 2 cases: (i) preliminary metadynamics runs for input into the method "Spectral gap optimization of order parameters" (SGOOP) and (ii) infrequent metadynamics runs [9] performed using different CVS.

### A. Preliminary metadynamics for input into SGOOP

#### 1. *Fullerene sterically constrained*

For these calculations, bias was added on $z$-coordinate as the only CV using gaussian width of 0.025 nm. Gaussians were deposited every 0.3 ps, with a starting height of 2 kJ/mol and gradually decreased on the basis of well-tempered metadynamics biasing factor $\gamma = 15$ [10]. Quartic restraining wall was used beyond $z = 1.7$. The effect of the walls on the potential of mean force was accounted for through reweighting [11].

#### 2. *Fullerene free to move in any direction*

For these calculations, bias was added on $z$-coordinate as the only CV using gaussian width of 0.025 nm. Gaussians were deposited every 0.3 ps, with a starting height of 2 kJ/mol and gradually decreased on the basis of well-tempered metadynamics biasing factor $\gamma = 15$ [10]. Two independent quartic restraining walls were used beyond $z = 1.7$ and $\rho \equiv \sqrt{x^2 + y^2} = 0.9$. The effect of the walls on the potential of mean force was accounted for through reweighting [11].

### B. Infrequent metadynamics for rate constants

These calculations were performed only for the case when the ligand was sterically constrained. For these calculations, bias was added on the respective trial CV using gaussian width of 0.01. Gaussians were deposited every 6 ps, with a starting height of 1.5 kJ/mol and gradually decreased on the basis of well-tempered metadynamics [10] biasing factor $\gamma = 12$ . Since these calculations were stopped after first escape (defined as reaching $z = 1.4$), no restraining walls were used.

## IV. SIMULATION DETAILS FOR SGOOP

### A. Input runs

As described in the main text, SGOOP needs a starting estimate of the stationary density. We obtained these using metadynamics with frequent metadynamics (Sec. III A). For the sterically constrained case, we show results obtained using starting metadynamics runs of durations 10, 15 and 20 ns, in order to demonstrate the convergence of the spectral gaps. For the constraint-free case, we show results obtained using starting metadynamics runs of durations 20 ns. Using runs of shorter (10 or 15 ns, as long as the ligand had escaped the cavity once) or longer (30, 40 or 50 ns, with multiple entry and exit events) gave identical results.

### B. Smoothening

The stationary density estimate obtained from metadynamics will have an inherent roughness depending on the number of bins used to grid the trial CV. Note that the current formulation of SGOOP [12] necessitates such a discretization in space. Thus, for any trial CV, there is an implicit smoothening of the stationary probability density $p(s)$, or equivalently, of the free energy $F(s) = -kTlog(p(s))$ that must be carried out. In order to remove any artifacts due to this operation, we performed calculations of spectral gap using different number of bins and report the averaged value so obtained. Specifically, for any trial CV $s$, we used 15, 20,...,50 bins. For each of these the spectral gap was normalized so that the input CV used in Sec. III A has a spectral gap of 1. The spectral gaps using various bins were then averaged to provide smoothening-independent estimates of the spectral gaps.


[1] J. Mondal, J. A. Morrone, and B. J. Berne, Proc. Natl. Acad. Sci. **110**, 13277 (2013).
[2] P. Tiwary, J. Mondal, J. A. Morrone, and B. J. Berne, Proc. Natl. Acad. Sci. (2015).
[3] W. L. Jorgensen, D. S. Maxwell, and J. Tirado-Rives, Journal of the American Chemical Society **118**, 11225 (1996).

[4] W. L. Jorgensen, J. Chandrasekhar, J. D. Madura, R. W. Impey, and M. L. Klein, J. Chem. Phys. **79**, 926 (1983).
[5] B. Hess, C. Kutzner, D. Van Der Spoel, and E. Lindahl, Journal of chemical theory and computation **4**, 435 (2008).
[6] G. A. Tribello, M. Bonomi, D. Branduardi, C. Camilloni, and G. Bussi, Comp. Phys. Comm. **185**, 604 (2014).
[7] G. Bussi, D. Donadio, and M. Parrinello, J. Chem. Phys. **126**, 014101 (2007).
[8] H. J. Berendsen, J. P. M. Postma, W. F. van Gunsteren, A. DiNola, and J. Haak, The Journal of chemical physics **81**, 3684 (1984).
[9] P. Tiwary and M. Parrinello, Phys. Rev. Lett. **111**, 230602 (2013).
[10] A. Barducci, G. Bussi, and M. Parrinello, Phys Rev Lett **100**, 020603 (2008).
[11] P. Tiwary and M. Parrinello, J. Phys. Chem. B **119**, 736 (2014).
[12] P. Tiwary and B. J. Berne, Proc. Natl. Acad. Sci. **113**, 2839 (2016).
